# Supplementary material for: CAM-Seg: A Continuous-valued Embedding Approach for Semantic Image Generation
Source: arXiv:2503.15617 source file (2025-03-19)
Supplement: Supplementary file 1 [file additional_info.tex]

\begin{table*}[!http]
\caption{zero shot domain adaptation}
\centering
\vspace{5ex}
\resizebox{2\columnwidth}{!}{

\begin{tabular}{l|ccccccccccccccccccc|c}
Dataset                                 & \begin{rotate}{90} Road\end{rotate}  & \begin{rotate}{90}Sidewalk\end{rotate}       & \begin{rotate}{90}Building\end{rotate} & \begin{rotate}{90}Wall\end{rotate}           & \begin{rotate}{90}Fence\end{rotate}          & \begin{rotate}{90}Pole\end{rotate}           & \begin{rotate}{90} TLight\end{rotate}  & \begin{rotate}{90} TSignal\end{rotate} & \begin{rotate}{90}Vtation\end{rotate} & \begin{rotate}{90}Terrain\end{rotate} & \begin{rotate}{90}Sky\end{rotate}   & \begin{rotate}{90}Person\end{rotate} & \begin{rotate}{90}Rider\end{rotate} & \begin{rotate}{90}Car\end{rotate}            & \begin{rotate}{90}Truck\end{rotate}          & \begin{rotate}{90}Bus\end{rotate}            & \begin{rotate}{90}Train\end{rotate}          & \begin{rotate}{90}Mcycle\end{rotate}    & \begin{rotate}{90}Bicycle\end{rotate}        & mIOU      \\

\hline
\hline
City & 96.40 & 77.89 & 84.61 & 25.00 & 17.99 & 31.34 & 34.02 & 49.06 & 87.00 & 60.16 & 92.83 & 55.72 & 24.49 & 89.50 & 27.15 & 48.97 & 21.30 & 16.49 & 42.58 & 51.71\\
Fog & 90.38 & 73.29 & 64.02 & 18.89 & 21.13 & 20.68 & 42.92 & 21.52 & 72.75 & 50.14 & 93.18 & 27.60 & 30.02 & 69.22 & 33.66 & 29.63 & 18.30 & 0.20 & 8.84 & 41.39\\
Night & 49.32 & 34.44 & 33.77 & 12.20 & 10.08 & 10.64 & 15.18 & 14.31 & 55.42 & 24.03 & 61.18 & 8.51 & 0.00 & 31.48 & 0.05 & 0.07 & 0.48 & 3.98 & 5.54 & 19.51\\
Rain & 76.95 & 48.64 & 67.83 & 11.74 & 13.80 & 21.05 & 31.91 & 21.99 & 83.13 & 50.34 & 94.56 & 23.35 & 9.56 & 60.70 & 4.27 & 15.12 & 2.08 & 0.23 & 4.79 & 33.79\\
snow & 82.79 & 53.19 & 48.76 & 16.34 & 11.53 & 14.56 & 33.62 & 25.06 & 49.59 & 24.38 & 90.64 & 22.82 & 1.91 & 54.26 & 5.44 & 1.22 & 39.87 & 0.09 & 1.39 & 30.39\\
\end{tabular}}
\end{table*}

\begin{table*}[!http]
\caption{Accuracy for context length 1024}
\centering
\vspace{5ex}
\resizebox{2\columnwidth}{!}{

\begin{tabular}{l|ccccccccccccccccccc|c}
Dataset                                 & \begin{rotate}{90} Road\end{rotate}  & \begin{rotate}{90}Sidewalk\end{rotate}       & \begin{rotate}{90}Building\end{rotate} & \begin{rotate}{90}Wall\end{rotate}           & \begin{rotate}{90}Fence\end{rotate}          & \begin{rotate}{90}Pole\end{rotate}           & \begin{rotate}{90} TLight\end{rotate}  & \begin{rotate}{90} TSignal\end{rotate} & \begin{rotate}{90}Vtation\end{rotate} & \begin{rotate}{90}Terrain\end{rotate} & \begin{rotate}{90}Sky\end{rotate}   & \begin{rotate}{90}Person\end{rotate} & \begin{rotate}{90}Rider\end{rotate} & \begin{rotate}{90}Car\end{rotate}            & \begin{rotate}{90}Truck\end{rotate}          & \begin{rotate}{90}Bus\end{rotate}            & \begin{rotate}{90}Train\end{rotate}          & \begin{rotate}{90}Mcycle\end{rotate}    & \begin{rotate}{90}Bicycle\end{rotate}        & AP      \\

\hline
\hline
City & 97.39 & 85.03 & 87.84 & 39.29 & 37.35 & 51.68 & 50.12 & 78.88 & 90.88 & 77.16 & 95.07 & 65.09 & 59.71 & 93.16 & 41.54 & 59.19 & 9.55 & 40.55 & 54.60 & 63.90\\
Kitti & 80.88 & 72.89 & 74.95 & 9.70 & 15.38 & 26.54 & 55.19 & 51.59 & 95.04 & 87.93 & 95.59 & 42.28 & 18.54 & 85.04 & 12.51 & 20.68 & 2.12 & 9.57 & 17.24 & 45.98\\
Fog & 93.36 & 82.20 & 56.26 & 22.45 & 23.84 & 21.47 & 53.97 & 33.55 & 91.10 & 74.81 & 97.68 & 28.74 & 32.73 & 79.17 & 20.12 & 29.18 & 19.38 & 1.72 & 10.05 & 45.88\\
Rain & 86.64 & 73.02 & 73.56 & 11.68 & 18.89 & 19.69 & 46.58 & 24.81 & 92.00 & 65.09 & 98.50 & 22.04 & 13.68 & 67.47 & 1.83 & 28.38 & 7.87 & 2.84 & 7.28 & 40.10\\
Snow & 83.35 & 70.01 & 45.74 & 17.16 & 16.04 & 15.13 & 40.59 & 33.82 & 91.93 & 59.67 & 96.40 & 24.02 & 0.27 & 60.09 & 6.18 & 7.74 & 35.22 & 1.05 & 1.50 & 37.15\\
Night & 81.30 & 78.46 & 27.09 & 28.12 & 31.03 & 15.39 & 0.11 & 30.68 & 91.62 & 52.67 & 97.80 & 11.51 & 1.04 & 45.94 & 0.11 & 0.06 & 3.57 & 2.61 & 8.19 & 31.96\\
Dark & 32.34 & 17.70 & 25.72 & 2.60 & 2.59 & 0.82 & 0.00 & 5.88 & 55.43 & 5.40 & 5.74 & 0.58 & 13.45 & 27.99 & 0.07 & 0.10 & 0.00 & 0.00 & 0.18 & 10.35\\
CAD & 38.37 & 56.08 & 22.97 & 0.93 & 7.23 & 11.61 & \textemdash{} & 5.54 & 84.31 & 73.37 & 92.52 & 8.69 & \textemdash{} & 31.30 & 1.70 & 0.47 & \textemdash{} & \textemdash{} & \textemdash{} & 31.08\\
\end{tabular}}
\end{table*}

\begin{table*}[!http]
\caption{Accuracy for context length 256}
\centering
\vspace{5ex}
\resizebox{2\columnwidth}{!}{

\begin{tabular}{l|ccccccccccccccccccc|c}
Dataset                                 & \begin{rotate}{90} Road\end{rotate}  & \begin{rotate}{90}Sidewalk\end{rotate}       & \begin{rotate}{90}Building\end{rotate} & \begin{rotate}{90}Wall\end{rotate}           & \begin{rotate}{90}Fence\end{rotate}          & \begin{rotate}{90}Pole\end{rotate}           & \begin{rotate}{90} TLight\end{rotate}  & \begin{rotate}{90} TSignal\end{rotate} & \begin{rotate}{90}Vtation\end{rotate} & \begin{rotate}{90}Terrain\end{rotate} & \begin{rotate}{90}Sky\end{rotate}   & \begin{rotate}{90}Person\end{rotate} & \begin{rotate}{90}Rider\end{rotate} & \begin{rotate}{90}Car\end{rotate}            & \begin{rotate}{90}Truck\end{rotate}          & \begin{rotate}{90}Bus\end{rotate}            & \begin{rotate}{90}Train\end{rotate}          & \begin{rotate}{90}Mcycle\end{rotate}    & \begin{rotate}{90}Bicycle\end{rotate}        & AP      \\

\hline
\hline
City & 96.88 & 81.89 & 86.08 & 41.85 & 36.32 & 42.65 & 33.61 & 65.53 & 88.90 & 72.42 & 93.98 & 56.85 & 47.19 & 91.25 & 41.98 & 42.01 & 40.97 & 22.55 & 49.11 & 59.58\\
Kitti & 75.50 & 66.72 & 66.87 & 10.55 & 19.10 & 19.07 & 40.26 & 31.66 & 93.01 & 87.81 & 94.97 & 30.61 & 14.01 & 80.18 & 8.65 & 22.44 & 1.53 & 5.43 & 12.83 & 41.12\\
Fog & 86.30 & 77.32 & 54.99 & 17.31 & 26.68 & 26.09 & 36.19 & 33.85 & 91.28 & 68.02 & 98.29 & 10.73 & 31.73 & 72.34 & 8.36 & 6.32 & 4.09 & 0.10 & 4.41 & 39.70\\
Rain & 82.33 & 70.52 & 64.47 & 9.71 & 17.78 & 21.48 & 43.02 & 23.71 & 91.24 & 64.10 & 98.45 & 16.30 & 10.70 & 54.63 & 1.45 & 35.28 & 6.91 & 1.42 & 11.77 & 38.17\\
Snow & 75.52 & 61.79 & 47.21 & 15.59 & 17.24 & 13.40 & 28.66 & 29.26 & 91.08 & 53.54 & 97.47 & 14.38 & 0.00 & 48.73 & 1.76 & 2.82 & 24.99 & 0.13 & 1.07 & 32.88\\
Night & 70.56 & 49.62 & 38.31 & 24.26 & 13.16 & 6.77 & 0.75 & 22.40 & 89.33 & 50.77 & 97.72 & 5.39 & 0.14 & 36.93 & 0.32 & 0.37 & 2.64 & 0.87 & 5.30 & 27.14\\
Dark & 38.87 & 37.18 & 24.65 & 2.65 & 2.92 & 1.36 & 0.00 & 0.00 & 70.46 & 8.68 & 0.00 & 1.04 & 0.00 & 39.78 & 0.29 & 0.35 & 0.00 & 0.00 & 1.33 & 12.08\\
CAD & 34.37 & 45.52 & 30.70 & 2.15 & 3.82 & 10.81 & \textemdash{} & 1.42 & 83.01 & 72.04 & 90.04 & 8.46 & \textemdash{} & 27.90 & 0.74 & 0.61 & \textemdash{} & \textemdash{} & \textemdash{} & 29.40\\
\end{tabular}}
\end{table*}

\begin{table*}[!http]
\caption{Result for salt and pepper noise Cityscape}
\centering
\vspace{5ex}
\resizebox{2\columnwidth}{!}{

\begin{tabular}{l|ccccccccccccccccccc|c}
Noise                                 & \begin{rotate}{90} Road\end{rotate}  & \begin{rotate}{90}Sidewalk\end{rotate}       & \begin{rotate}{90}Building\end{rotate} & \begin{rotate}{90}Wall\end{rotate}           & \begin{rotate}{90}Fence\end{rotate}          & \begin{rotate}{90}Pole\end{rotate}           & \begin{rotate}{90} TLight\end{rotate}  & \begin{rotate}{90} TSignal\end{rotate} & \begin{rotate}{90}Vtation\end{rotate} & \begin{rotate}{90}Terrain\end{rotate} & \begin{rotate}{90}Sky\end{rotate}   & \begin{rotate}{90}Person\end{rotate} & \begin{rotate}{90}Rider\end{rotate} & \begin{rotate}{90}Car\end{rotate}            & \begin{rotate}{90}Truck\end{rotate}          & \begin{rotate}{90}Bus\end{rotate}            & \begin{rotate}{90}Train\end{rotate}          & \begin{rotate}{90}Mcycle\end{rotate}    & \begin{rotate}{90}Bicycle\end{rotate}        & AP      \\
\hline
\hline
0\% & 98.06 & 86.36 & 89.23 & 47.26 & 43.44 & 60.10 & 62.97 & 82.55 & 92.69 & 80.27 & 95.98 & 70.89 & 64.30 & 94.02 & 44.99 & 66.59 & 43.73 & 48.27 & 62.66 & 70.23\\
1\% & 97.64 & 83.53 & 87.63 & 43.04 & 37.82 & 54.11 & 54.94 & 77.11 & 91.26 & 77.54 & 95.38 & 67.25 & 58.58 & 92.94 & 42.90 & 63.16 & 36.24 & 40.15 & 55.43 & 66.14\\
2\% & 97.55 & 82.83 & 87.35 & 41.88 & 36.35 & 53.40 & 54.06 & 76.26 & 91.07 & 76.32 & 95.31 & 66.62 & 57.21 & 92.80 & 42.12 & 62.09 & 34.45 & 38.39 & 53.06 & 65.22\\
5\% & 97.33 & 81.93 & 86.98 & 40.01 & 34.18 & 51.64 & 52.24 & 74.64 & 90.64 & 75.04 & 95.18 & 65.73 & 55.60 & 92.57 & 41.59 & 61.09 & 31.51 & 35.85 & 50.10 & 63.89\\
10\% & 97.08 & 80.61 & 86.28 & 37.50 & 31.46 & 49.19 & 49.81 & 72.53 & 90.23 & 74.49 & 95.15 & 64.60 & 53.98 & 92.28 & 39.57 & 59.53 & 27.22 & 35.28 & 46.62 & 62.28\\
25\% & 96.41 & 77.26 & 82.91 & 31.70 & 26.97 & 44.07 & 43.74 & 67.82 & 89.61 & 73.36 & 95.20 & 62.23 & 50.73 & 91.96 & 33.93 & 56.03 & 21.34 & 31.81 & 40.21 & 58.80\\
50\% & 90.43 & 68.36 & 73.35 & 17.24 & 18.61 & 33.92 & 39.81 & 66.35 & 89.37 & 72.74 & 95.18 & 58.83 & 49.56 & 91.20 & 24.23 & 49.34 & 20.83 & 29.42 & 32.82 & 53.77\\
60\% & 43.95 & 5.86 & 27.48 & 0.66 & 1.04 & 2.03 & 0.38 & 7.08 & 53.48 & 0.81 & 9.05 & 2.05 & 0.00 & 9.42 & 0.49 & 1.15 & 0.38 & 0.00 & 0.93 & 8.75\\
70\% & 37.89 & 5.18 & 20.74 & 0.69 & 0.68 & 1.27 & 0.04 & 2.96 & 25.35 & 1.24 & 2.18 & 1.04 & 0.00 & 6.82 & 0.52 & 0.27 & 0.01 & 0.00 & 0.60 & 5.66\\
80\% & 35.95 & 5.09 & 19.53 & 0.75 & 0.69 & 1.21 & 0.13 & 0.99 & 17.75 & 0.95 & 1.96 & 0.92 & 0.11 & 6.59 & 0.44 & 0.37 & 0.37 & 0.00 & 0.64 & 4.97\\

\end{tabular}}
\end{table*}

\begin{table*}[!http]
\caption{Result for Motion Blur}
\centering
\vspace{5ex}
\resizebox{2\columnwidth}{!}{

\begin{tabular}{l|ccccccccccccccccccc|c}
Kernel                                 & \begin{rotate}{90} Road\end{rotate}  & \begin{rotate}{90}Sidewalk\end{rotate}       & \begin{rotate}{90}Building\end{rotate} & \begin{rotate}{90}Wall\end{rotate}           & \begin{rotate}{90}Fence\end{rotate}          & \begin{rotate}{90}Pole\end{rotate}           & \begin{rotate}{90} TLight\end{rotate}  & \begin{rotate}{90} TSignal\end{rotate} & \begin{rotate}{90}Vtation\end{rotate} & \begin{rotate}{90}Terrain\end{rotate} & \begin{rotate}{90}Sky\end{rotate}   & \begin{rotate}{90}Person\end{rotate} & \begin{rotate}{90}Rider\end{rotate} & \begin{rotate}{90}Car\end{rotate}            & \begin{rotate}{90}Truck\end{rotate}          & \begin{rotate}{90}Bus\end{rotate}            & \begin{rotate}{90}Train\end{rotate}          & \begin{rotate}{90}Mcycle\end{rotate}    & \begin{rotate}{90}Bicycle\end{rotate}        & AP      \\
\hline
\hline
3 & 97.98 & 86.32 & 89.07 & 46.97 & 41.93 & 58.91 & 61.34 & 81.66 & 92.58 & 80.14 & 96.06 & 70.91 & 62.86 & 93.89 & 44.78 & 66.16 & 41.06 & 44.95 & 60.96 & 69.40\\
9 & 97.87 & 85.84 & 88.73 & 46.91 & 41.19 & 57.26 & 60.20 & 80.12 & 92.33 & 79.49 & 96.02 & 69.58 & 61.46 & 93.70 & 43.97 & 65.53 & 39.08 & 41.88 & 59.29 & 68.45\\
15 & 97.79 & 85.30 & 88.41 & 46.31 & 39.96 & 55.49 & 58.19 & 78.99 & 92.07 & 79.14 & 95.83 & 68.26 & 59.97 & 93.52 & 43.31 & 64.87 & 37.57 & 41.13 & 57.60 & 67.56\\
21 & 97.70 & 84.83 & 87.99 & 45.63 & 38.84 & 52.96 & 55.95 & 77.50 & 91.76 & 78.42 & 95.77 & 67.09 & 58.19 & 93.26 & 42.23 & 64.02 & 35.63 & 39.61 & 55.59 & 66.47\\
35 & 97.44 & 83.87 & 87.06 & 44.31 & 37.22 & 47.80 & 52.68 & 74.29 & 91.22 & 77.27 & 95.56 & 65.37 & 56.11 & 92.63 & 40.51 & 62.42 & 33.33 & 33.77 & 52.54 & 64.49\\
51 & 97.01 & 82.67 & 85.82 & 43.06 & 35.41 & 43.31 & 49.20 & 71.04 & 90.71 & 76.04 & 95.24 & 63.85 & 53.78 & 91.92 & 38.43 & 60.41 & 29.95 & 30.11 & 49.87 & 62.52\\
75 & 96.34 & 81.24 & 84.24 & 41.65 & 32.99 & 39.24 & 45.81 & 68.26 & 90.21 & 74.51 & 94.76 & 62.74 & 52.07 & 91.20 & 36.16 & 57.94 & 25.48 & 27.90 & 47.64 & 60.55\\
105 & 95.49 & 79.62 & 82.53 & 39.51 & 30.06 & 35.59 & 43.19 & 66.34 & 89.67 & 72.46 & 94.13 & 61.77 & 50.67 & 90.53 & 33.81 & 54.98 & 21.10 & 26.14 & 45.60 & 58.59\\
151 & 86.13 & 51.92 & 67.29 & 18.17 & 8.22 & 3.95 & 1.41 & 23.31 & 83.07 & 50.26 & 83.58 & 31.01 & 1.13 & 82.40 & 15.00 & 30.74 & 3.01 & 0.34 & 14.26 & 34.48\\
221 & 82.92 & 42.03 & 63.93 & 10.27 & 6.18 & 3.59 & 1.27 & 19.00 & 82.03 & 39.53 & 79.90 & 22.91 & 0.93 & 80.77 & 10.33 & 25.18 & 1.72 & 0.25 & 9.94 & 30.67\\
\end{tabular}}
\end{table*}

\begin{table*}[!http]
\caption{Result for Gaussian Noise}
\centering
\vspace{5ex}
\resizebox{2\columnwidth}{!}{

\begin{tabular}{l|ccccccccccccccccccc|c}
Std                                 & \begin{rotate}{90} Road\end{rotate}  & \begin{rotate}{90}Sidewalk\end{rotate}       & \begin{rotate}{90}Building\end{rotate} & \begin{rotate}{90}Wall\end{rotate}           & \begin{rotate}{90}Fence\end{rotate}          & \begin{rotate}{90}Pole\end{rotate}           & \begin{rotate}{90} TLight\end{rotate}  & \begin{rotate}{90} TSignal\end{rotate} & \begin{rotate}{90}Vtation\end{rotate} & \begin{rotate}{90}Terrain\end{rotate} & \begin{rotate}{90}Sky\end{rotate}   & \begin{rotate}{90}Person\end{rotate} & \begin{rotate}{90}Rider\end{rotate} & \begin{rotate}{90}Car\end{rotate}            & \begin{rotate}{90}Truck\end{rotate}          & \begin{rotate}{90}Bus\end{rotate}            & \begin{rotate}{90}Train\end{rotate}          & \begin{rotate}{90}Mcycle\end{rotate}    & \begin{rotate}{90}Bicycle\end{rotate}        & AP      \\
\hline
\hline
5 & 97.98 & 85.84 & 88.95 & 46.86 & 42.83 & 59.11 & 59.85 & 81.72 & 92.37 & 79.37 & 95.80 & 70.20 & 62.54 & 93.81 & 43.72 & 65.93 & 41.41 & 43.40 & 60.97 & 69.09\\
10 & 97.98 & 85.83 & 88.95 & 46.46 & 42.94 & 58.95 & 60.28 & 81.62 & 92.39 & 79.43 & 95.83 & 70.13 & 62.27 & 93.82 & 43.39 & 65.64 & 41.56 & 43.98 & 60.83 & 69.07\\
20 & 97.98 & 85.81 & 88.93 & 43.84 & 42.71 & 58.65 & 60.70 & 81.57 & 92.39 & 79.34 & 95.81 & 70.19 & 62.61 & 93.85 & 43.58 & 65.87 & 41.87 & 43.89 & 60.79 & 68.97\\
30 & 97.99 & 85.82 & 88.92 & 44.39 & 42.79 & 58.67 & 60.67 & 81.57 & 92.40 & 79.32 & 95.81 & 70.20 & 62.56 & 93.85 & 43.89 & 65.85 & 41.68 & 44.03 & 60.83 & 69.01\\
50 & 97.99 & 85.82 & 88.92 & 44.83 & 42.77 & 58.67 & 60.79 & 81.54 & 92.40 & 79.32 & 95.81 & 70.16 & 62.42 & 93.84 & 43.95 & 65.95 & 41.73 & 44.02 & 60.88 & 69.04\\
100 & 97.98 & 85.81 & 88.91 & 45.14 & 42.73 & 58.69 & 60.79 & 81.52 & 92.39 & 79.28 & 95.82 & 70.14 & 62.54 & 93.84 & 44.04 & 66.01 & 41.72 & 44.08 & 60.91 & 69.07\\
\end{tabular}}
\end{table*}

\begin{table*}[!http]
\caption{Result for Gaussian Blur}
\centering
\vspace{5ex}
\resizebox{2\columnwidth}{!}{

\begin{tabular}{l|ccccccccccccccccccc|c}
Sigma                                 & \begin{rotate}{90} Road\end{rotate}  & \begin{rotate}{90}Sidewalk\end{rotate}       & \begin{rotate}{90}Building\end{rotate} & \begin{rotate}{90}Wall\end{rotate}           & \begin{rotate}{90}Fence\end{rotate}          & \begin{rotate}{90}Pole\end{rotate}           & \begin{rotate}{90} TLight\end{rotate}  & \begin{rotate}{90} TSignal\end{rotate} & \begin{rotate}{90}Vtation\end{rotate} & \begin{rotate}{90}Terrain\end{rotate} & \begin{rotate}{90}Sky\end{rotate}   & \begin{rotate}{90}Person\end{rotate} & \begin{rotate}{90}Rider\end{rotate} & \begin{rotate}{90}Car\end{rotate}            & \begin{rotate}{90}Truck\end{rotate}          & \begin{rotate}{90}Bus\end{rotate}            & \begin{rotate}{90}Train\end{rotate}          & \begin{rotate}{90}Mcycle\end{rotate}    & \begin{rotate}{90}Bicycle\end{rotate}        & AP      \\
\hline
\hline
1& 98.00 & 85.83 & 88.84 & 47.24 & 41.52 & 58.56 & 61.82 & 81.48 & 92.43 & 79.72 & 96.04 & 70.04 & 62.14 & 94.03 & 44.51 & 66.16 & 40.18 & 42.16 & 60.04 & 68.99\\
5 & 97.54 & 81.98 & 87.05 & 44.85 & 34.01 & 53.74 & 55.12 & 76.12 & 91.60 & 76.36 & 95.59 & 63.44 & 57.74 & 93.47 & 39.97 & 64.07 & 33.58 & 36.23 & 50.60 & 64.90\\
11 & 97.55 & 81.80 & 86.94 & 44.82 & 34.05 & 53.52 & 55.72 & 76.07 & 91.62 & 76.35 & 95.50 & 63.10 & 57.12 & 93.53 & 40.38 & 63.92 & 33.53 & 35.88 & 50.54 & 64.84\\
25 & 97.55 & 81.73 & 86.88 & 44.73 & 34.03 & 53.31 & 55.76 & 76.16 & 91.63 & 76.39 & 95.44 & 62.94 & 57.09 & 93.58 & 40.63 & 63.89 & 33.72 & 35.93 & 50.51 & 64.84\\
50 & 97.78 & 83.63 & 87.81 & 45.83 & 37.79 & 55.79 & 58.90 & 78.70 & 92.02 & 77.94 & 95.69 & 66.11 & 59.56 & 93.83 & 42.78 & 64.99 & 36.68 & 39.31 & 55.76 & 66.89\\
\end{tabular}}
\end{table*}

\begin{table*}[!http]
\caption{Result for brightness Variation}
\centering
\vspace{5ex}
\resizebox{2\columnwidth}{!}{

\begin{tabular}{l|ccccccccccccccccccc|c}
Factor                                 & \begin{rotate}{90} Road\end{rotate}  & \begin{rotate}{90}Sidewalk\end{rotate}       & \begin{rotate}{90}Building\end{rotate} & \begin{rotate}{90}Wall\end{rotate}           & \begin{rotate}{90}Fence\end{rotate}          & \begin{rotate}{90}Pole\end{rotate}           & \begin{rotate}{90} TLight\end{rotate}  & \begin{rotate}{90} TSignal\end{rotate} & \begin{rotate}{90}Vtation\end{rotate} & \begin{rotate}{90}Terrain\end{rotate} & \begin{rotate}{90}Sky\end{rotate}   & \begin{rotate}{90}Person\end{rotate} & \begin{rotate}{90}Rider\end{rotate} & \begin{rotate}{90}Car\end{rotate}            & \begin{rotate}{90}Truck\end{rotate}          & \begin{rotate}{90}Bus\end{rotate}            & \begin{rotate}{90}Train\end{rotate}          & \begin{rotate}{90}Mcycle\end{rotate}    & \begin{rotate}{90}Bicycle\end{rotate}        & AP      \\
\hline
\hline
0.5 & 98.01 & 85.75 & 89.01 & 46.42 & 43.24 & 58.50 & 60.59 & 81.77 & 92.38 & 80.19 & 95.09 & 70.77 & 62.87 & 94.07 & 46.70 & 67.19 & 44.13 & 41.83 & 62.78 & 69.54\\
0.75 & 98.02 & 85.95 & 89.07 & 44.86 & 43.60 & 58.77 & 61.60 & 81.98 & 92.50 & 80.11 & 95.42 & 70.81 & 62.78 & 94.06 & 44.91 & 66.71 & 43.94 & 43.74 & 62.72 & 69.56\\
1.25 & 98.03 & 86.09 & 89.08 & 43.03 & 43.57 & 59.00 & 61.80 & 82.11 & 92.60 & 80.12 & 94.97 & 70.90 & 63.28 & 94.02 & 44.66 & 66.39 & 42.73 & 45.00 & 62.50 & 69.47\\
1.5 & 98.04 & 86.15 & 89.04 & 43.64 & 43.73 & 59.11 & 61.72 & 82.19 & 92.66 & 80.20 & 94.40 & 70.97 & 63.34 & 93.95 & 44.05 & 66.08 & 41.23 & 46.11 & 62.27 & 69.41\\
\end{tabular}}
\end{table*}

\begin{table*}[!http]
\caption{Result for Contrast Variation}
\centering
\vspace{5ex}
\resizebox{2\columnwidth}{!}{

\begin{tabular}{l|ccccccccccccccccccc|c}
Factor                                 & \begin{rotate}{90} Road\end{rotate}  & \begin{rotate}{90}Sidewalk\end{rotate}       & \begin{rotate}{90}Building\end{rotate} & \begin{rotate}{90}Wall\end{rotate}           & \begin{rotate}{90}Fence\end{rotate}          & \begin{rotate}{90}Pole\end{rotate}           & \begin{rotate}{90} TLight\end{rotate}  & \begin{rotate}{90} TSignal\end{rotate} & \begin{rotate}{90}Vtation\end{rotate} & \begin{rotate}{90}Terrain\end{rotate} & \begin{rotate}{90}Sky\end{rotate}   & \begin{rotate}{90}Person\end{rotate} & \begin{rotate}{90}Rider\end{rotate} & \begin{rotate}{90}Car\end{rotate}            & \begin{rotate}{90}Truck\end{rotate}          & \begin{rotate}{90}Bus\end{rotate}            & \begin{rotate}{90}Train\end{rotate}          & \begin{rotate}{90}Mcycle\end{rotate}    & \begin{rotate}{90}Bicycle\end{rotate}        & AP      \\
\hline
\hline
0.5 & 98.01 & 86.24 & 88.87 & 46.87 & 42.91 & 57.97 & 60.33 & 81.28 & 92.38 & 78.28 & 95.54 & 70.56 & 62.71 & 94.25 & 45.20 & 67.47 & 43.81 & 41.24 & 61.46 & 69.23\\
0.75 & 98.04 & 86.33 & 89.00 & 47.01 & 43.24 & 58.61 & 61.14 & 81.64 & 92.49 & 78.94 & 95.64 & 70.75 & 63.28 & 94.17 & 44.71 & 67.18 & 43.57 & 42.94 & 61.78 & 69.50\\
1.25 & 98.04 & 86.28 & 89.04 & 46.83 & 43.25 & 59.00 & 61.54 & 81.87 & 92.55 & 79.33 & 95.39 & 70.76 & 63.16 & 94.09 & 45.03 & 66.79 & 41.88 & 42.50 & 62.00 & 69.44\\
1.5 & 98.03 & 86.25 & 88.90 & 45.87 & 42.91 & 58.94 & 61.43 & 81.88 & 92.50 & 79.57 & 95.09 & 70.63 & 63.23 & 93.94 & 45.11 & 66.03 & 40.93 & 34.00 & 61.66 & 68.78\\
\end{tabular}}
\end{table*}

\begin{table*}[!http]
\caption{Result for Saturation Variation}
\centering
\vspace{5ex}
\resizebox{2\columnwidth}{!}{

\begin{tabular}{l|ccccccccccccccccccc|c}
Factor                                 & \begin{rotate}{90} Road\end{rotate}  & \begin{rotate}{90}Sidewalk\end{rotate}       & \begin{rotate}{90}Building\end{rotate} & \begin{rotate}{90}Wall\end{rotate}           & \begin{rotate}{90}Fence\end{rotate}          & \begin{rotate}{90}Pole\end{rotate}           & \begin{rotate}{90} TLight\end{rotate}  & \begin{rotate}{90} TSignal\end{rotate} & \begin{rotate}{90}Vtation\end{rotate} & \begin{rotate}{90}Terrain\end{rotate} & \begin{rotate}{90}Sky\end{rotate}   & \begin{rotate}{90}Person\end{rotate} & \begin{rotate}{90}Rider\end{rotate} & \begin{rotate}{90}Car\end{rotate}            & \begin{rotate}{90}Truck\end{rotate}          & \begin{rotate}{90}Bus\end{rotate}            & \begin{rotate}{90}Train\end{rotate}          & \begin{rotate}{90}Mcycle\end{rotate}    & \begin{rotate}{90}Bicycle\end{rotate}        & AP      \\
\hline
\hline
0 & 97.26 & 78.11 & 81.92 & 23.30 & 38.19 & 53.83 & 52.34 & 69.61 & 93.60 & 43.32 & 93.92 & 68.91 & 63.87 & 92.69 & 36.49 & 59.70 & 11.22 & 48.06 & 57.44 & 61.25\\
0.5 & 98.04 & 85.95 & 88.92 & 46.17 & 42.99 & 59.13 & 61.59 & 81.88 & 92.70 & 78.92 & 96.00 & 70.65 & 63.86 & 94.08 & 45.42 & 66.39 & 39.23 & 48.32 & 62.15 & 69.60\\
1.5 & 98.06 & 86.11 & 89.00 & 46.36 & 42.89 & 59.29 & 62.04 & 81.85 & 92.69 & 78.94 & 96.11 & 70.74 & 63.94 & 94.10 & 45.06 & 66.25 & 40.87 & 47.08 & 62.24 & 69.66 \\
2 & 98.12 & 86.29 & 89.03 & 46.06 & 42.15 & 59.39 & 62.85 & 81.32 & 92.65 & 77.46 & 96.54 & 70.74 & 64.13 & 94.29 & 43.83 & 65.90 & 42.03 & 43.17 & 61.94 & 69.36\\
\end{tabular}}
\end{table*}

\begin{table*}[!http]
\caption{Result for Hue Variation}
\centering
\vspace{5ex}
\resizebox{2\columnwidth}{!}{

\begin{tabular}{l|ccccccccccccccccccc|c}
Factor                                 & \begin{rotate}{90} Road\end{rotate}  & \begin{rotate}{90}Sidewalk\end{rotate}       & \begin{rotate}{90}Building\end{rotate} & \begin{rotate}{90}Wall\end{rotate}           & \begin{rotate}{90}Fence\end{rotate}          & \begin{rotate}{90}Pole\end{rotate}           & \begin{rotate}{90} TLight\end{rotate}  & \begin{rotate}{90} TSignal\end{rotate} & \begin{rotate}{90}Vtation\end{rotate} & \begin{rotate}{90}Terrain\end{rotate} & \begin{rotate}{90}Sky\end{rotate}   & \begin{rotate}{90}Person\end{rotate} & \begin{rotate}{90}Rider\end{rotate} & \begin{rotate}{90}Car\end{rotate}            & \begin{rotate}{90}Truck\end{rotate}          & \begin{rotate}{90}Bus\end{rotate}            & \begin{rotate}{90}Train\end{rotate}          & \begin{rotate}{90}Mcycle\end{rotate}    & \begin{rotate}{90}Bicycle\end{rotate}        & AP      \\
\hline
\hline
-0.2 & 96.69 & 79.05 & 78.28 & 28.01 & 33.71 & 48.07 & 46.25 & 64.78 & 90.97 & 53.55 & 96.32 & 60.34 & 59.36 & 92.77 & 29.53 & 52.22 & 18.97 & 37.98 & 52.94 & 58.94\\
-0.1 & 97.27 & 81.15 & 82.74 & 33.42 & 36.87 & 52.82 & 52.46 & 70.22 & 91.87 & 66.51 & 96.55 & 64.72 & 62.54 & 93.42 & 37.24 & 57.77 & 23.26 & 40.62 & 56.34 & 63.04\\
0.1 & 97.48 & 83.00 & 84.71 & 32.61 & 37.75 & 54.10 & 55.46 & 73.15 & 91.63 & 66.91 & 96.20 & 66.33 & 62.02 & 93.51 & 41.18 & 59.56 & 29.46 & 38.16 & 57.88 & 64.27\\
0.2 & 97.48 & 83.49 & 85.15 & 31.85 & 36.62 & 53.09 & 54.48 & 70.44 & 90.32 & 61.22 & 95.87 & 65.82 & 61.18 & 93.05 & 37.92 & 53.58 & 22.13 & 36.45 & 57.63 & 62.51\\
\end{tabular}}
\end{table*}

\begin{table}[!http]
\caption{Effect of Salt and Pepper Noise}
\centering
\begin{tabular}{lc|ccc}
Noise Ratio & AP & AP\textsuperscript{F} & AP\textsuperscript{C} & AP\textsuperscript{R}\\
\hline
\hline
0\% & 70.23 &  92.46 &  63.00 &  61.58\\
1\% & 66.14 &  91.09 &  59.37 &  55.09\\
2\% & 65.22 &  90.82 &  58.50 &  53.65\\
5\% & 63.89 &  90.41 &  57.25 &  51.58\\
10\% & 62.28 &  89.87 &  55.58 &  49.28\\
25\% & 58.80 &  88.28 &  52.03 &  44.53\\
50\% & 53.77 &  83.34 &  45.25 &  41.16\\
60\% & 8.75 &  27.96 &   2.36 &   1.42\\
70\% & 5.66 &  18.27 &   1.75 &   0.55\\
80\% & 4.97 &  16.06 &   1.65 &   0.37\\
\end{tabular}
\end{table}

\begin{table}[!http]
\caption{Effect of Motion blur}
\centering
\begin{tabular}{lc|ccc}
Kernel size & AP & AP\textsuperscript{F} & AP\textsuperscript{C} & AP\textsuperscript{R}\\
\hline
\hline
0 & 70.23 &  92.46 &  63.00 &  61.58\\
3 & 69.40 &  92.40 &  62.50 &  59.86\\
9 & 68.44 &  92.16 &  61.73 &  58.22\\
15 & 67.56 &  91.88 &  60.86 &  56.90\\
21 & 66.47 &  91.61 &  59.78 &  55.21\\
35 & 64.49 &  91.03 &  57.87 &  52.16\\
51 & 62.52 &  90.29 &  56.00 &  49.19\\
75 & 60.55 &  89.36 &  54.07 &  46.44\\
105 & 58.59 &  88.29 &  51.96 &  44.00\\
151 & 34.48 &  74.40 &  29.86 &  10.60\\
221 & 30.67 &  70.16 &  24.80 &   8.33\\
\end{tabular}
\end{table}

\begin{table}[!http]
\caption{Effect of Gaussian Noise}
\centering
\begin{tabular}{lc|ccc}
std & AP & AP\textsuperscript{F} & AP\textsuperscript{C} & AP\textsuperscript{R}\\
\hline
\hline
0 & 70.23 &  92.46 &  63.00 &  61.58\\
5 & 69.09 &  92.19 &  62.27 &  59.40\\
10 & 69.07 &  92.20 &  62.16 &  59.45\\
20 & 68.97 &  92.18 &  61.74 &  59.61\\
30 & 69.01 &  92.19 &  61.87 &  59.60\\
50 & 69.04 &  92.19 &  61.93 &  59.62\\
100 & 69.07 &  92.18 &  61.98 &  59.65\\
\end{tabular}
\end{table}

\begin{table}[!http]
\caption{Effect of Gaussian Blur}
\centering
\begin{tabular}{lc|ccc}
sigma & AP & AP\textsuperscript{F} & AP\textsuperscript{C} & AP\textsuperscript{R}\\
\hline
\hline
0 & 70.23 &  92.46 &  63.00 &  61.58\\
1 & 68.99 &  92.23 &  62.23 &  59.14\\
5 & 64.90 &  90.75 &  57.98 &  53.35\\
11 & 64.84 &  90.68 &  57.96 &  53.25\\
25 & 64.84 &  90.65 &  57.94 &  53.29\\
50 & 66.89 &  91.39 &  60.01 &  56.27\\
\end{tabular}
\end{table}

\begin{table}[!http]
\caption{Effect of Brightness Variation}
\centering
\begin{tabular}{lc|ccc}
factor & AP & AP\textsuperscript{F} & AP\textsuperscript{C} & AP\textsuperscript{R}\\
\hline
\hline
0.5 & 69.54 &  92.05 &  62.84 &  60.17\\
0.75 & 69.56 &  92.19 &  62.45 &  60.50\\
1 & 70.23 &  92.46 &  63.00 &  61.58\\
1.25 & 69.47 &  92.15 &  62.19 &  60.54\\
1.5 & 69.41 &  92.06 &  62.24 &  60.42\\
\end{tabular}
\end{table}

\begin{table}[!http]
\caption{Effect of Contrast Variation}
\centering
\begin{tabular}{lc|ccc}
factor & AP & AP\textsuperscript{F} & AP\textsuperscript{C} & AP\textsuperscript{R}\\
\hline
\hline
0.5 & 69.23 &  92.21 &  62.29 &  59.76\\
0.75 & 69.50 &  92.30 &  62.49 &  60.22\\
1 & 70.23 &  92.46 &  63.00 &  61.58\\
1.25 & 69.44 &  92.26 &  62.61 &  59.96\\
1.5 & 68.78 &  92.15 &  62.42 &  58.45\\
\end{tabular}
\end{table}

\begin{table}[!http]
\caption{Effect of Saturation Variation}
\centering
\begin{tabular}{lc|ccc}
factor & AP & AP\textsuperscript{F} & AP\textsuperscript{C} & AP\textsuperscript{R}\\
\hline
\hline
0 & 61.25 &  88.96 &  50.96 &  51.75\\
0.5 & 69.60 &  92.32 &  62.48 &  60.49\\
1 & 70.23 &  92.46 &  63.00 &  61.58\\
1.5 & 69.66 &  92.39 &  62.48 &  60.61\\
2 & 69.36 &  92.53 &  61.99 &  60.19\\
\end{tabular}
\end{table}

\begin{table}[!http]
\caption{Effect of Hue Variation}
\centering
\begin{tabular}{lc|ccc}
factor & AP & AP\textsuperscript{F} & AP\textsuperscript{C} & AP\textsuperscript{R}\\
\hline
\hline
-0.2 & 58.94 &  88.26 &  49.43 &  47.50\\
-0.1 & 63.04 &  89.92 &  55.00 &  51.89\\
0 & 70.23 &  92.46 &  63.00 &  61.58\\
0.1 & 64.27 &  90.60 &  56.06 &  53.67\\
0.2 & 62.51 &  90.46 &  54.22 &  50.84\\
\end{tabular}
\end{table}

\begin{table}[!http]
\caption{Context length variation(size)}
% \label{tab:context lenght}
\centering
\resizebox{\columnwidth}{!}{

\begin{tabular}{lccc|ccc|ccc}
& \multicolumn{3}{c|}{2304} & \multicolumn{3}{|c|}{1024} & \multicolumn{3}{|c}{256}\\
% \cline{2-10}
Dataset & AP\textsuperscript{S} & AP\textsuperscript{M} & AP\textsuperscript{L} & AP\textsuperscript{S} & AP\textsuperscript{M} & AP\textsuperscript{L} & AP\textsuperscript{S} & AP\textsuperscript{M} & AP\textsuperscript{L}\\
\hline
\hline
City & 68.16 &  57.67 &  84.26 & 61.10 &  47.99 &  81.81 & 49.17 &  46.31 &  80.29\\
KITTI & 45.23 &  26.49 &  75.54 & 38.83 &  23.22 &  73.85 & 27.12 &  21.45 &  70.78\\
Fog & 42.94 &  32.11 &  78.33 & 34.09 &  26.21 &  73.98 & 27.72 &  17.47 &  70.50\\
Rain & 32.71 &  20.79 &  73.92 & 25.36 &  19.22 &  71.50 & 23.04 &  18.46 &  68.69\\
Snow & 26.38 &  20.20 &  71.40 & 22.77 &  18.26 &  66.32 & 17.14 &  13.82 &  63.17\\
Night & 14.10 &  11.00 &  68.18 & 11.75 &  13.07 &  65.29 & 7.09 &   8.51 &  60.08\\
Dark &  2.23 &   3.67 &  22.01 & 4.15 &   4.42 &  20.70 & 0.48 &   6.38 &  26.07\\
CAD &  9.13 &  14.44 &  57.63 & 8.61 &  10.18 &  52.65 & 6.90 &   8.27 &  51.12\\
\end{tabular}}
\end{table}

\begin{table}[!http]
\caption{Context length variation(frequency)}
\label{tab:contextlenght}
\centering
\resizebox{\columnwidth}{!}{

\begin{tabular}{lccc|ccc|ccc}
& \multicolumn{3}{c|}{2304} & \multicolumn{3}{|c|}{1024} & \multicolumn{3}{|c}{256}\\
% \cline{2-10}
Dataset & AP\textsuperscript{F} & AP\textsuperscript{C} & AP\textsuperscript{R} & AP\textsuperscript{F} & AP\textsuperscript{C} & AP\textsuperscript{R} & AP\textsuperscript{F} & AP\textsuperscript{C} & AP\textsuperscript{R}\\
\hline
\hline
City & 92.46 &  63.00 &  61.58 & 91.24 &  57.90 &  50.37 & 89.55 &  54.76 &  43.00\\
KITTI & 85.82 &  43.02 &  30.01 & 83.87 &  39.91 &  24.99 & 79.41 &  36.57 &  18.31\\
Fog & 88.18 &  47.96 &  30.17 & 84.12 &  38.66 &  25.80 & 81.64 &  32.79 &  16.67\\
Rain & 86.77 &  34.21 &  21.89 & 84.74 &  29.53 &  18.78 & 81.40 &  26.49 &  18.97\\
Snow & 81.37 &  32.98 &  19.34 & 77.49 &  28.33 &  17.17 & 74.61 &  23.52 &  12.42\\
Night & 79.56 &  26.43 &   5.99 & 75.25 &  26.40 &   6.61 & 69.11 &  19.66 &   4.64\\
Dark & 29.74 &   4.94 &   1.10 & 27.39 &   5.72 &   2.80 & 34.23 &   8.10 &   0.24\\
CAD & 64.54 &  23.10 &   2.08 & 58.85 &  19.26 &   3.00 & 56.73 &  17.99 &   1.01\\
\end{tabular}}
\end{table}
